# Supplementary material for: DivIL: Unveiling and Addressing Over-Invariance for Out-of- Distribution Generalization
Source: arXiv:2502.12413 source file (2025-05-22)
Supplement: Supplementary file 1 [file appendix.tex]

\section{appendix}
% In this section, we present two reasons: 1) strong regularization constraints and 2) feature diversity loss.
\subsection{Theorem}
\begin{theorem}[Class Suppression in supervised Contrastive Learning~\cite{features_CL}] \label{class-collapse}
    Considering a linear model with $p$ outputs, which has weights $\mathbf{W}\in \mathbb{R}^{p\times d}$ and bias $\mathbf{b}\in R^{p} $ where $p\ge 3 $, we can define the function represented by this model as $f_{\mathbf{\Theta}}=\mathbf{Wx}+\mathbf{b}$, where $\mathbf{\Theta}\in R^{p\times (d+1)}$ as the concatenated parameter $[\mathbf{W}\ \mathbf{b}]$.
    Let \( \mathbf{\Theta}^{**} = [\mathbf{W}^{**}, \mathbf{b}^{**}] \) be the minimum norm minimizer of the contrastive learning loss \( L_{CL} \). Suppose \( \mathbf{\Theta}^{**} \) minimizes the loss as follows:
    \[
    \mathbf{\Theta}^{**} = \arg\min_{\mathbf{\Theta}^{*}} \|\mathbf{\Theta}^{*}\|_F \quad \text{such that} \quad \mathbf{\Theta}^{*} \in \arg\min_{\mathbf{\Theta}} L_{CL}(\mathbf{\Theta}).
    \]
    With high probability (at least \( 1 - O\left(\frac{m^2}{n^2 d}\right) = 1 - o(1) \)), \( \mathbf{W}^{**} \) has no alignment with the subclass feature \( v_2 \), meaning:
    \[
    \|\mathbf{W}^{**} v_2\| = 0.
    \]
    Thus, \textbf{class collapse} occurs at test time, meaning no linear classifier can predict subclass labels better than random guessing.
\end{theorem}

\begin{theorem}[Feature Suppression in Unsupervised Contrastive Learning~\cite{features_CL}] \label{feature-suppression}
   Let \( p \leq K \), where \( p \) represents the number of dimensions in the encoded feature space and \( K \) the total number of features. Define the tuple \( \mathcal{L} = \{1, \phi_1^2, \phi_2^2, \dots, \phi_K^2\} \), where each \( \phi_i^2 \) represents the variance of the features. If \( \phi_1^2 \) (class feature) is not among the \( p \)-largest elements of \( \mathcal{L} \), then with high probability \( 1 - O\left(\frac{m^2}{n^2 d}\right) = 1 - o(1) \):
        (1) There exists a global minimizer \( \mathbf{\Theta}^{*} \) such that \( \|W^{*} v_1\| = \Omega(1) \),
        (2) However, the minimum norm minimizer \( \mathbf{\Theta}^{**} \) satisfies \( \|W^{**} v_1\| = 0 \).
This suggests that the \textbf{class feature} is suppressed when the embedding space is too limited to capture all the feature dimensions, and only the most discriminative features are retained in the encoded space. 
\end{theorem}

\begin{theorem}[Alleviate over-invariance via \ours]
    Let \( \mathbf{\Theta}^{**} \) be the minimum norm minimizer of the joint contrastive loss \( L_{joint, \beta} \) defined as:
    \[
    L_{joint, \beta}(\mathbf{\Theta}) = \beta L_{SCL}(\mathbf{\Theta}) + (1 - \beta) L_{UCL}(\mathbf{\Theta}),
    \]
    where \( L_{SCL} \) and \( L_{UCL} \) are supervised and unsupervised contrastive losses, respectively, and \( \beta \in (0, 1) \). Assume without loss of generality that \( \phi_3^2 \geq \phi_4^2 \geq \dots \geq \phi_K^2 \), and the class feature variance \( \phi_1^2 \) is smaller than the variance of irrelevant features \( \phi_2^2 \). In this scenario, the minimum norm minimizer of \( L_{SCL} \) suffers from \textbf{class collapse} (Theorem \ref{class-collapse}), and the minimum norm minimizer of \( L_{UCL} \ref{feature-suppression} \).
    However, for a suitable \( \beta \), the minimum norm minimizer of \( L_{joint, \beta} \) avoids both phenomena and learns both class and subclass features effectively.  
\end{theorem}

\section{Full Details of the Background}
\label{sec:prelim_appdx}
We give a more detailed background introduction about GNNs and Invariant Learning in this section.

\textbf{Graph Neural Networks.} Let $G=(A,X)$ denote a graph with $n$ nodes and $m$ edges,
where $A \in \{0,1\}^{n\times n}$ is the adjacency matrix, and $X\in \R^{n \times d}$ is the node feature matrix
with a node feature dimension of $d$.
In graph classification, we are given a set of $N$ graphs $\{G_i\}_{i=1}^N\subseteq \gG$
and their labels $\{Y_i\}_{i=1}^N\subseteq\gY=\R^c$ from $c$ classes.
Then, we train a GNN $\rho \circ h$ with an encoder $h:\gG\rightarrow\R^h$ that learns a meaningful representation $h_G$ for each graph $G$ to help predict their labels $y_G=\rho(h_G)$ with a downstream classifier $\rho:\R^h\rightarrow\gY$.
The representation $h_G$ is typically obtained by performing pooling with a $\text{READOUT}$ function on the learned node representations:
\begin{equation}
    \label{eq:gnn_pooling}
    h_G = \text{READOUT}(\{h^{(K)}_u|u\in V\}),
\end{equation}
where the $\text{READOUT}$ is a permutation invariant function (e.g., $\text{SUM}$, $\text{MEAN}$, $\text{MAX}$)~\citep{gin},
and $h^{(K)}_u$ stands for the node representation of $u\in V$ at $K$-th layer that is obtained by neighbor aggregation:
\begin{equation}
    \label{eq:gnn}
    h^{(K)}_u = \sigma(W_K\cdot a(\{h^{(K-1)}_v\}| v\in\mathcal{N}(u)\cup\{u\})),
\end{equation}
where $\mathcal{N}(u)$ is the set of neighbors of node $u$,
$\sigma(\cdot)$ is an activation function, e.g., $\text{ReLU}$, and $a(\cdot)$ is an aggregation function over neighbors, e.g., $\text{MEAN}$.

\paragraph{Graph generation process.}
This work focuses on graph classification, while the results generalize
to node classification as well using the same setting as in~\citet{eerm}.
Specifically,
we are given a set of graph datasets $\dataset=\{\dataset_e\}_e$ collected from multiple environments $\envall$.
Samples $(G^e_i, Y^e_i)\in \dataset^e$ from the same
environment are considered as drawn independently from an identical distribution $\sP^e$.
We consider the graph generation process proposed
by~\citet{ciga} that covers a broad case of graph distribution shifts.
Fig.~\ref{fig:scm_appdx} shows the full graph generation process considered in~\citet{ciga}.
The generation of the observed graph $G$ and labels $Y$
are controlled by a set of latent causal variable $C$ and spurious variable $S$, i.e.,
\[G\coloneqq f_\gen(C,S).\]
$C$ and $S$ control the generation of $G$ by controlling the underlying invariant subgraph $G_c$
and spurious subgraph $G_s$, respectively.
Since $S$ can be affected by the environment $E$,
the correlation between $Y$, $S$ and $G_s$ can change arbitrarily
when the environment changes.
$C$ and $S$ control the generation of the underlying invariant subgraph $G_c$
and spurious subgraph $G_s$, respectively.
Since $S$ can be affected by the environment $E$,
the correlation between $Y$, $S$ and $G_s$ can change arbitrarily
when the environment changes.
Besides, the latent interaction among $C$, $S$ and $Y$
can be further categorized into \emph{Full Informative Invariant Features} (\emph{FIIF})
when $Y\ind S|C$ and \emph{Partially Informative Invariant Features} (\emph{PIIF}) when $Y \not\ind S|C$. Furthermore, PIIF and FIIF shifts can be mixed together and yield \emph{Mixed Informative Invariant Features} (\emph{MIIF}), as shown in Fig.~\ref{fig:scm_appdx}.
We refer interested readers to~\citet{ciga} for a detailed introduction of the graph generation process.

\paragraph{Invariant graph representation learning.}
To tackle the OOD generalization challenge
on graphs from Fig.~\ref{fig:scm_appdx},
the existing invariant graph learning approaches generically
aim to identify the underlying invariant subgraph $G_c$ to predict the label $Y$~\citep{eerm,ciga}.
Specifically, the goal of OOD generalization on graphs
is to learn an \emph{invariant GNN} $f\coloneqq f_c\circ g$,
which is composed of two modules:
a) a featurizer $g:\gG\rightarrow\gG_c$ that extracts the invariant subgraph $G_c$;
b) a classifier $f_c:\gG_c\rightarrow\gY$ that predicts the label $Y$ based on the extracted $G_c$,
where $\gG_c$ refers to the space of subgraphs of $\gG$.
The learning objectives of $f_c$ and $g$ are formulated as
%\vspace{-0.05in}
\begin{equation}
    \label{eq:inv_cond_appdx}
    \text{$\max$}_{f_c, \; g} \ I(\pred{G}_{c};Y), \ \text{s.t.}\ \pred{G}_{c}\ind E,\ \pred{G}_{c}=g(G).
\end{equation}
Since $E$ is not observed, many strategies are proposed to
impose the independence of $\pred{G}_c$ and $E$.
A common approach is to augment the environment information.
For example, based on the estimated invariant subgraphs $\pred{G}_c$ and spurious subgraphs $\pred{G}_s$,
\citet{dir,grea,eerm} proposed to generate new environments, while \citet{moleood,gil} proposed to infer the underlying environment labels.
% \citet{moleood} propose a variational framework to infer the environment labels.
However, we show that it is fundamentally impossible to augment faithful environment information in Sec.~\ref{sec:env_aug_failure}.
\citet{gib,gsat,dps,lri} adopt graph information bottleneck to tackle FIIF graph shifts, and they cannot generalize to PIIF shifts.
Our works focuses on PIIF shifts, as it is more challenging when without environment labels~\citep{zin}.
\citet{disc} generalized~\citep{ldd} to tackle severe graph biases, i.e., when $H(S|Y)< H(C|Y)$.
\citet{ciga} proposed a contrastive framework to tackle both
FIIF and PIFF graph shifts, but limited to $H(S|Y)> H(C|Y)$.
However, in practice it is usually unknown whether $H(S|Y)< H(C|Y)$ or $H(S|Y)> H(C|Y)$ without environment information.

\paragraph{More OOD generalization on graphs.}
In addition to the aforementioned invariant learning approaches, \citet{size_gen1,size_gen2,size_gen3} study the OOD generalization as extrapolation from small graphs to larger graphs in the task of graph classification and link prediction. In contrast, we study OOD generalization against various graph distribution shifts formulated in Fig.~\ref{fig:scm_appdx}. In addition to the standard OOD generalization tasks studied in this paper, \citet{nn_extrapo,OOD_CLRS} study the OOD generalization in tasks of algorithmic reasoning on graphs. \citet{graph_ttt} study the test-time adaption in the graph regime. \citet{shape_matching} study the 3D shape matching under the presence of noises.

\paragraph{Invariant learning without environment labels.}
There are also plentiful studies in invariant learning without environment labels.
\citet{eiil} proposed a minmax formulation to infer the environment labels.
\citet{hrm} proposed a self-boosting framework based on the estimated invariant and variant features.
\citet{jtt,cnc} proposed to infer labels based the predictions of an ERM trained model.
However, \citet{zin} found failure cases in Euclidean data
where it is impossible to identify the invariant features without given environment labels.
Moreover, as the OOD generalization on graphs is fundamentally more difficult than Euclidean data~\citep{ciga}, the question about the feasibility of learning invariant subgraphs without environment labels remains unanswered.
